# Supplementary material for: PanJoin: A Partition-based Adaptive Stream Join
Source: arXiv:1811.05065 source file (2018-11-13)
Supplement: Supplementary file 1 [file appendix.tex]

\appendix
%Appendix A
%\section{Headings in Appendices}
